# Supplementary material for: Autonomous heterogeneous catalyst discovery with a self-evolving multi-agent digital twin
Source: arXiv:2606.05050 source file (2026-07-09)
Supplement: Supplementary file 1 [file si-xr.tex]

% Auto-generated by gen-si-xr.py -- do not edit by hand.
% Regenerate after compiling si.tex: python3 gen-si-xr.py
\makeatletter
\expandafter\gdef\csname r@si-LastBibItem\endcsname{{12}{50}{}{section*.115}{}}
\expandafter\gdef\csname r@si-eq:bandit_update\endcsname{{S3}{33}{}{equation.60}{}}
\expandafter\gdef\csname r@si-eq:episode_reward\endcsname{{S4}{33}{}{equation.61}{}}
\expandafter\gdef\csname r@si-eq:iter_reward\endcsname{{S2}{33}{}{equation.58}{}}
\expandafter\gdef\csname r@si-eq:retrieval_scorer\endcsname{{S1}{32}{}{equation.56}{}}
\expandafter\gdef\csname r@si-fig:neb_attempt_ladder\endcsname{{S1}{17}{NEB attempt-ladder outcome distribution}{figure.18}{}}
\expandafter\gdef\csname r@si-fig:si_c3h6_network\endcsname{{S4}{26}{*CO to C$_3$H$_6$ pathway network}{figure.35}{}}
\expandafter\gdef\csname r@si-fig:si_case_bank\endcsname{{S8}{34}{RL case-bank composition}{figure.64}{}}
\expandafter\gdef\csname r@si-fig:si_ch4_network\endcsname{{S3}{25}{*CO to CH$_4$ pathway network}{figure.33}{}}
\expandafter\gdef\csname r@si-fig:si_cu1o3_caz\endcsname{{S11}{40}{Cu$_1$-O$_3$/ZrO$_2$ CAZ series}{figure.85}{}}
\expandafter\gdef\csname r@si-fig:si_ni5ga3_tdep\endcsname{{S12}{41}{Ni$_5$Ga$_3$ T-dependent CO/CH$_3$OH ratio}{figure.88}{}}
\expandafter\gdef\csname r@si-fig:si_ni_tiox_fe\endcsname{{S14}{43}{Ni@TiO$_x$ PDH free-energy profile}{figure.98}{}}
\expandafter\gdef\csname r@si-fig:si_pdh_cost\endcsname{{S15}{47}{PDH discovery candidates: material cost analysis}{figure.111}{}}
\expandafter\gdef\csname r@si-fig:si_pdmo_multi_p\endcsname{{S13}{41}{hcp-PdMo CO$_2$ conversion}{figure.91}{}}
\expandafter\gdef\csname r@si-fig:si_phase1_care\endcsname{{S6}{28}{Phase~1 vs.\ CARE cost}{figure.44}{}}
\expandafter\gdef\csname r@si-fig:si_pos_neg_ablation\endcsname{{S9}{35}{Positive vs.\ negative ablation}{figure.69}{}}
\expandafter\gdef\csname r@si-fig:si_ru_b5_nh3\endcsname{{S10}{39}{Ru B$_5$ NH$_3$ TOF comparison}{figure.82}{}}
\expandafter\gdef\csname r@si-fig:si_scaling\endcsname{{S5}{28}{UniMech vs.\ CARE scaling}{figure.42}{}}
\expandafter\gdef\csname r@si-fig:si_throughput\endcsname{{S16}{49}{Per-structure CatDT wall time}{figure.114}{}}
\expandafter\gdef\csname r@si-fig:si_unimech_detail\endcsname{{S2}{22}{UniMech three-phase pipeline}{figure.25}{}}
\expandafter\gdef\csname r@si-fig:thermo_db_stats\endcsname{{S7}{29}{CatDT molecule database statistics}{figure.47}{}}
\expandafter\gdef\csname r@si-note:architecture\endcsname{{1}{7}{}{section*.5}{}}
\expandafter\gdef\csname r@si-note:benchmark_details\endcsname{{5}{39}{}{section*.79}{}}
\expandafter\gdef\csname r@si-note:endpoints\endcsname{{1.3}{16}{}{section*.14}{}}
\expandafter\gdef\csname r@si-note:harness\endcsname{{1.2}{13}{}{section*.12}{}}
\expandafter\gdef\csname r@si-note:hyperparams\endcsname{{1.1}{10}{}{section*.9}{}}
\expandafter\gdef\csname r@si-note:memento_schema\endcsname{{1.4}{18}{}{section*.20}{}}
\expandafter\gdef\csname r@si-note:pdh_cost\endcsname{{6}{45}{}{section*.102}{}}
\expandafter\gdef\csname r@si-note:pdh_rounds_detail\endcsname{{6.1}{45}{}{section*.103}{}}
\expandafter\gdef\csname r@si-note:rl_loop\endcsname{{3}{30}{}{section*.50}{}}
\expandafter\gdef\csname r@si-note:skill_ablation\endcsname{{4}{36}{}{section*.72}{}}
\expandafter\gdef\csname r@si-note:thermo_db\endcsname{{2.4}{28}{}{section*.45}{}}
\expandafter\gdef\csname r@si-note:throughput\endcsname{{7}{48}{}{section*.112}{}}
\expandafter\gdef\csname r@si-note:unimech\endcsname{{2}{22}{}{section*.23}{}}
\expandafter\gdef\csname r@si-ssec:bandit\endcsname{{3.4}{33}{}{section*.59}{}}
\expandafter\gdef\csname r@si-ssec:benchmark_summary\endcsname{{5.9}{43}{}{section*.100}{}}
\expandafter\gdef\csname r@si-ssec:cu1o3_span\endcsname{{5.2}{40}{}{section*.83}{}}
\expandafter\gdef\csname r@si-ssec:iter_reward\endcsname{{3.3}{33}{}{section*.57}{}}
\expandafter\gdef\csname r@si-ssec:mo2c_table\endcsname{{5.6}{42}{}{section*.93}{}}
\expandafter\gdef\csname r@si-ssec:mos2_vacancy\endcsname{{5.5}{42}{}{section*.92}{}}
\expandafter\gdef\csname r@si-ssec:ni5ga3_tdep\endcsname{{5.3}{40}{}{section*.86}{}}
\expandafter\gdef\csname r@si-ssec:nitiox_ea\endcsname{{5.7}{42}{}{section*.96}{}}
\expandafter\gdef\csname r@si-ssec:nitiox_selectivity\endcsname{{5.8}{43}{}{section*.99}{}}
\expandafter\gdef\csname r@si-ssec:pdh_cost_analysis\endcsname{{6.2}{46}{}{section*.106}{}}
\expandafter\gdef\csname r@si-ssec:pdmo_multi_p\endcsname{{5.4}{41}{}{section*.89}{}}
\expandafter\gdef\csname r@si-ssec:rl_ablation\endcsname{{3.6}{35}{}{section*.65}{}}
\expandafter\gdef\csname r@si-ssec:rl_protocol\endcsname{{3.5}{34}{}{section*.62}{}}
\expandafter\gdef\csname r@si-ssec:ru_b5_nh3\endcsname{{5.1}{39}{}{section*.80}{}}
\expandafter\gdef\csname r@si-ssec:scorer\endcsname{{3.2}{32}{}{section*.55}{}}
\expandafter\gdef\csname r@si-ssec:two_stage\endcsname{{3.1}{31}{}{section*.51}{}}
\expandafter\gdef\csname r@si-tab:ablation\endcsname{{S16}{36}{\textbf {Coarse-grained progression of memory and RL components} (subset of Table~\ref {tab:rl_ablation_full} rows; cumulative additions on top of the stateless agent)}{table.71}{}}
\expandafter\gdef\csname r@si-tab:agents\endcsname{{S2}{10}{\textbf {The eight CatDT agents.}}{table.8}{}}
\expandafter\gdef\csname r@si-tab:benchmark_summary\endcsname{{S19}{44}{\textbf {Quantitative comparison of CatDT predictions with experiment and literature.}}{table.101}{}}
\expandafter\gdef\csname r@si-tab:harness_budgets\endcsname{{S5}{14}{Agent harness budgets and timeouts}{table.13}{}}
\expandafter\gdef\csname r@si-tab:hyperparams\endcsname{{S3}{10}{CatDT pipeline hyperparameter compendium}{table.10}{}}
\expandafter\gdef\csname r@si-tab:memento_schema\endcsname{{S8}{19}{Memory-bank and cache schemas}{table.21}{}}
\expandafter\gdef\csname r@si-tab:mo2c_rates\endcsname{{S18}{42}{\textbf {Predicted vs.\ experimental product formation rates over 2D-Mo$_2$C} at 230~$^\circ $C and 25~bar (units: mg~h$^{-1}$~g$_\text {cat}^{-1}$)}{table.95}{}}
\expandafter\gdef\csname r@si-tab:neb_attempt_ladder\endcsname{{S6}{17}{CatDT adaptive NEB attempt ladder}{table.16}{}}
\expandafter\gdef\csname r@si-tab:neb_validator\endcsname{{S7}{18}{Post-NEB validation gates}{table.19}{}}
\expandafter\gdef\csname r@si-tab:pathways_ch4\endcsname{{S11}{25}{\textbf {All 13 pathways discovered by Agent~M1 for *CO $\to $ CH$_4$(g) on Ni(111).} (G) = agent-guided; (S) = systematic}{table.31}{}}
\expandafter\gdef\csname r@si-tab:pathways_summary\endcsname{{S13}{27}{\textbf {Agent~M1 pathway discovery summary across 14 Fischer--Tropsch targets on Ni(111).}}{table.40}{}}
\expandafter\gdef\csname r@si-tab:rl_ablation_full\endcsname{{S15}{35}{\textbf {Staged ablation of the Agent~4/5 reinforcement stack} on the 50-case holdout set at the final checkpoint. ``Knowledge'' and ``Skill'' refer to the distilled banks individually; ``Full RL stack'' adds the episode-level bandit and the parametric retriever on top of the three banks (Case + Knowledge + Skill). The eight configurations listed here are the same eight visualised in main Fig.~4f}{table.67}{}}
\expandafter\gdef\csname r@si-tab:scaling\endcsname{{S12}{27}{\textbf {Network scaling comparison (Agent~M1 vs.\ CARE).}}{table.38}{}}
\expandafter\gdef\csname r@si-tab:skill_ablation\endcsname{{S17}{38}{\textbf {Sound-gated skill-ablation results} across the twelve Fig.~\ref {fig:architecture}b prompts (five reps per arm). ``Sound pass@5'' counts only runs that produce the deliverable with a real ML/DFT potential and physically correct energetics; P8 and P9 require no atomistic potential and are judged on method correctness. Median wall time is the per-prompt median of the full run wall clock (agent reasoning plus tool execution); runs hitting the one-hour watchdog enter at 60~min. The dominant Group~N failure mode per prompt is detailed in the failure taxonomy below}{table.77}{}}
\expandafter\gdef\csname r@si-tab:thermo_db_composition\endcsname{{S14}{30}{569-species molecule database breakdown}{table.49}{}}
\expandafter\gdef\csname r@si-tab:tools_full\endcsname{{S1}{7}{\textbf {Complete CAMEL FunctionTool registry (27 tools).}}{table.6}{}}
\expandafter\gdef\csname r@si-tab:unimech_ops\endcsname{{S10}{23}{\textbf {Agent~M1 elementary operation categories.}}{table.28}{}}
\makeatother
